# Supplementary material for: Excitonic Effects in Absorption Spectra of Carbon Dioxide Reduction Photocatalysts
Source: arXiv:2103.08384 source file (2021-03-15)
Supplement: Supplementary file 1 [file Supplementary_Information.pdf]

# Supplementary Information: Excitonic Effects in Absorption Spectra of Carbon Dioxide Reduction Photocatalysts

Tathagata Biswas* and Arunima K. Singh†
*Department of Physics, Arizona State University, Tempe AZ 85287*

* tbiswas3@asu.edu
† arunimasingh@asu.edu

## I. STRUCTURAL DETAILS

| mp-id | Formula | SG | This Work | | | | | | | Materials Project | | | | | | |
|---|---|---|---|---|---|---|---|---|---|---|---|---|---|---|---|---|
| | | | $a$ | $b$ | $c$ | $\alpha$ | $\beta$ | $\gamma$ | $E_g$ | $a$ | $b$ | $c$ | $\alpha$ | $\beta$ | $\gamma$ | $E_g$ |
| mp-2657 | $TiO_2$ | $P4_2/mnm$ | 2.96 | 4.61 | 4.61 | 90.00 | 90.00 | 90.00 | 1.83 | 2.98 | 4.60 | 4.60 | 90.00 | 90.00 | 90.00 | 1.81 |
| mp-34688 | $TiO_2$ | $C2/c$ | 3.94 | 3.94 | 4.58 | 109.04 | 109.04 | 90.56 | 2.22 | 3.79 | 3.79 | 3.79 | 110.34 | 110.34 | 90.00 | 2.04 |
| mp-390 | $TiO_2$ | $I4_1/amd$ | 3.80 | 3.80 | 5.47 | 110.31 | 110.31 | 90.00 | 2.07 | 3.84 | 3.84 | 5.53 | 110.30 | 110.30 | 90.00 | 2.14 |
| mp-5229 | $SrTiO_3$ | $Pm\bar{3}m$ | 3.91 | 3.91 | 3.91 | 90.00 | 90.00 | 90.00 | 1.94 | 3.90 | 3.90 | 3.90 | 90.00 | 90.00 | 90.00 | 1.86 |
| mp-4170 | $NaTaO_3$ | $Pm\bar{3}m$ | 3.95 | 3.95 | 3.95 | 90.00 | 90.00 | 90.02 | 2.46 | 3.92 | 3.92 | 3.92 | 90.00 | 90.00 | 90.03 | 2.34 |
| mp-556489 | $Ta_2SnO_6$ | $Cc$ | 4.88 | 5.55 | 8.90 | 90.58 | 105.90 | 90.00 | 2.10 | 4.87 | 5.55 | 8.90 | 90.57 | 105.89 | 90.00 | 2.37 |
| mp-20194 | $CeO_2$ | $Fm\bar{3}m$ | 3.85 | 3.85 | 3.85 | 60.00 | 60.00 | 60.00 | 2.19 | 3.83 | 3.83 | 3.83 | 60.00 | 60.00 | 60.00 | 1.88 |
| mp-36734 | $CeThO_4$ | $P4/mmm$ | 3.92 | 7.83 | 6.78 | 30.01 | 54.72 | 59.99 | 2.02 | 3.92 | 7.84 | 6.79 | 30.00 | 54.74 | 60.00 | 1.68 |
| mp-8789 | $Ca_4As_2O$ | $I4/mmm$ | 4.52 | 4.52 | 8.30 | 105.78 | 105.78 | 90.00 | 1.29 | 4.54 | 4.54 | 8.36 | 105.74 | 105.74 | 90.00 | 1.23 |
| mp-2172 | AlAs | $F\bar{4}3m$ | 4.05 | 4.05 | 4.05 | 60.00 | 60.00 | 60.00 | 1.62 | 4.00 | 4.00 | 4.00 | 60.00 | 60.00 | 60.00 | 1.50 |
| mp-8881 | AlAs | $P6_3mc$ | 4.04 | 4.04 | 6.62 | 90.00 | 90.00 | 120.00 | 1.82 | 3.98 | 3.98 | 6.50 | 90.00 | 90.00 | 120.00 | 1.68 |
| mp-1863 | SiAs | $C2/m$ | 3.72 | 8.29 | 9.64 | 105.35 | 90.00 | 102.97 | 1.27 | 3.67 | 8.20 | 9.53 | 105.58 | 90.00 | 102.93 | 1.48 |
| mp-27776 | $Cd_2AsCl_2$ | $P2_1/c$ | 7.93 | 8.05 | 9.18 | 90.00 | 90.00 | 118.22 | 1.06 | 7.86 | 8.03 | 9.19 | 90.00 | 90.00 | 117.98 | 1.05 |
| mp-1009087 | BeSiAs2 | $I\bar{4}2d$ | 5.37 | 5.37 | 6.53 | 114.27 | 114.27 | 90.00 | 1.09 | 5.98 | 5.98 | 6.98 | 115.38 | 115.38 | 90.00 | 1.02 |
| mp-1016197 | $MgSiAs_2$ | $I\bar{4}2d$ | 5.93 | 5.93 | 6.87 | 115.61 | 115.61 | 90.00 | 1.39 | 5.98 | 5.98 | 6.98 | 115.38 | 115.38 | 90.00 | 1.30 |
| mp-12558 | LiMgAs | $F\bar{4}3m$ | 4.37 | 4.37 | 4.37 | 60.00 | 60.00 | 60.00 | 1.55 | 4.38 | 4.38 | 4.38 | 60.00 | 60.00 | 60.00 | 1.46 |
| mp-961685 | NaCaAs | $F\bar{4}3m$ | 4.87 | 4.87 | 4.87 | 60.00 | 60.00 | 60.00 | 1.83 | 4.75 | 4.75 | 4.75 | 60.00 | 60.00 | 60.00 | 1.57 |
| mp-569454 | CdHgAsBr | $Pmma$ | 5.17 | 8.93 | 9.80 | 90.00 | 90.00 | 90.00 | 0.00 | 4.70 | 8.79 | 9.78 | 90.00 | 90.00 | 90.00 | 0.98 |
| mp-2624 | AlSb | $F\bar{4}3m$ | 4.34 | 4.34 | 4.34 | 60.00 | 60.00 | 60.00 | 1.30 | 4.34 | 4.34 | 4.34 | 60.00 | 60.00 | 60.00 | 1.24 |
| mp-9274 | $Rb_3Sb_2Au_3$ | $R\bar{3}m$ | 8.17 | 8.17 | 8.17 | 46.53 | 46.53 | 46.53 | 1.13 | 8.13 | 8.13 | 8.13 | 46.68 | 46.68 | 46.68 | 1.27 |
| mp-1634 | $MoSe_2$ | $P6_3/mmc$ | 3.33 | 3.33 | 13.17 | 90.00 | 90.00 | 120.00 | 0.97 | 3.29 | 3.29 | 12.90 | 90.00 | 90.00 | 120.00 | 1.49 |
| mp-1018807 | $MoSe_2$ | $P6_3/mmc$ | 3.32 | 3.32 | 13.06 | 90.00 | 90.00 | 120.00 | 0.95 | 3.28 | 3.28 | 12.92 | 90.00 | 90.00 | 120.00 | 1.24 |
| mp-7581 | $MoSe_2$ | $R3m$ | 6.87 | 6.87 | 6.87 | 28.06 | 28.06 | 28.06 | 1.07 | 6.74 | 6.74 | 6.74 | 28.28 | 28.28 | 28.28 | 1.43 |
| mp-1821 | $WSe_2$ | $P6_3/mmc$ | 3.31 | 3.31 | 13.04 | 90.00 | 90.00 | 120.00 | 1.06 | 3.28 | 3.28 | 12.96 | 90.00 | 90.00 | 120.00 | 1.53 |
| mp-15776 | $Zn(GaSe_2)_2$ | $I\bar{4}$ | 5.60 | 5.60 | 6.79 | 114.37 | 114.37 | 90.00 | 1.43 | 5.50 | 5.50 | 6.73 | 114.10 | 114.10 | 90.00 | 1.36 |
| mp-574620 | $CsYZnSe_3$ | $Cmcm$ | 4.14 | 8.17 | 10.93 | 90.00 | 90.00 | 104.67 | 1.94 | 4.14 | 8.17 | 10.93 | 90.00 | 90.00 | 104.67 | 2.12 |
| mp-510283 | $CsGaSe_3$ | $P2_1/c$ | 6.81 | 7.84 | 13.26 | 90.00 | 90.00 | 106.44 | 1.66 | 6.71 | 7.73 | 13.01 | 90.00 | 90.00 | 106.39 | 1.69 |
| mp-1943 | GaSe | $P6_3/mmc$ | 3.80 | 3.80 | 15.73 | 90.00 | 90.00 | 120.00 | 0.56 | 3.75 | 3.75 | 15.94 | 90.00 | 90.00 | 120.00 | 1.21 |
| mp-11342 | GaSe | $R3m$ | 8.34 | 8.34 | 8.34 | 26.34 | 26.34 | 26.34 | 0.72 | 8.26 | 8.26 | 8.26 | 26.22 | 26.22 | 26.22 | 1.29 |
| mp-1340 | $Ga_2Se_3$ | $Cc$ | 6.71 | 6.69 | 6.77 | 80.96 | 60.33 | 71.49 | 0.17 | 6.66 | 6.66 | 6.71 | 81.12 | 60.24 | 71.88 | 1.01 |
| mp-28423 | $Ga_2TeSe_2$ | $I4_1md$ | 7.43 | 7.43 | 7.41 | 120.08 | 120.08 | 90.00 | 1.58 | 7.26 | 7.26 | 7.42 | 119.28 | 119.28 | 90.00 | 1.58 |
| mp-567386 | $Cs_2Cd_3Te_4$ | $Ibam$ | 6.74 | 10.73 | 10.73 | 75.64 | 71.68 | 71.68 | 1.61 | 6.67 | 10.61 | 10.61 | 75.60 | 71.69 | 71.69 | 1.55 |
| mp-12491 | $CsLaCdTe_3$ | $Cmcm$ | 4.66 | 8.66 | 12.17 | 90.00 | 90.00 | 105.60 | 1.62 | 4.64 | 8.67 | 12.17 | 90.00 | 90.00 | 105.52 | 1.72 |
| mp-20782 | $LiInTe_2$ | $I\bar{4}2d$ | 6.47 | 6.47 | 7.82 | 114.43 | 114.43 | 90.00 | 1.40 | 6.31 | 6.31 | 7.63 | 114.41 | 114.41 | 90.00 | 1.37 |
| mp-22255 | $RbInTe_2$ | $I4/mcm$ | 7.32 | 7.32 | 7.32 | 105.14 | 105.14 | 118.53 | 1.01 | 7.24 | 7.24 | 7.24 | 105.02 | 105.02 | 118.79 | 1.29 |
| mp-35663 | $Sr(InTe_2)_2$ | $I4/m$ | 7.13 | 7.13 | 7.13 | 104.50 | 104.50 | 119.94 | 0.88 | 6.87 | 6.87 | 6.87 | 106.02 | 106.02 | 116.62 | 1.20 |
| mp-9008 | RbTeAu | $Pmma$ | 5.05 | 5.98 | 7.28 | 90.00 | 90.00 | 90.00 | 1.05 | 5.08 | 5.94 | 7.21 | 90.00 | 90.00 | 90.00 | 1.10 |
| mp-571195 | ZnTe | $P3_1$ | 4.36 | 4.36 | 10.31 | 90.00 | 90.00 | 120.00 | 0.92 | 4.04 | 4.05 | 9.34 | 90.00 | 90.00 | 120.00 | 1.04 |
| mp-8884 | ZnTe | $P6_3mc$ | 4.27 | 4.27 | 6.99 | 90.00 | 90.00 | 120.00 | 1.38 | 4.27 | 4.27 | 6.99 | 90.00 | 90.00 | 120.00 | 1.08 |
| mp-2176 | ZnTe | $F\bar{4}3m$ | 4.32 | 4.32 | 4.32 | 60.00 | 60.00 | 60.00 | 1.16 | 4.40 | 4.40 | 4.40 | 60.00 | 60.00 | 60.00 | 1.05 |
| mp-15777 | $Zn(GaTe_2)_2$ | $I\bar{4}$ | 6.14 | 6.14 | 7.50 | 114.14 | 114.14 | 90.00 | 0.68 | 5.94 | 5.94 | 7.27 | 114.10 | 114.10 | 90.00 | 1.00 |
| mp-13949 | $Cd(GaTe_2)_2$ | $I\bar{4}$ | 6.21 | 6.21 | 7.39 | 114.82 | 114.82 | 90.00 | 1.01 | 6.09 | 6.09 | 7.31 | 114.63 | 114.63 | 90.00 | 1.02 |
| mp-542812 | GaTe | $C2/m$ | 4.14 | 9.05 | 10.62 | 104.21 | 90.00 | 103.21 | 1.04 | 4.08 | 8.94 | 10.46 | 104.11 | 90.00 | 103.18 | 1.09 |
| mp-1779 | YbTe | $Fm\bar{3}m$ | 4.46 | 4.46 | 4.46 | 60.00 | 60.00 | 60.00 | 1.54 | 4.49 | 4.49 | 4.49 | 60.00 | 60.00 | 60.00 | 1.51 |
| mp-27449 | GaTeCl | $Pnnm$ | 4.13 | 5.90 | 14.59 | 90.00 | 90.00 | 90.00 | 2.04 | 4.08 | 5.85 | 14.47 | 90.00 | 90.00 | 90.00 | 2.16 |
| mp-29236 | InTeBr | $P2_1/c$ | 7.46 | 7.70 | 8.32 | 90.00 | 115.45 | 90.00 | 1.51 | 7.35 | 7.58 | 8.17 | 90.00 | 115.23 | 90.00 | 1.72 |
| mp-33723 | BiTeBr | $P3m1$ | 4.36 | 4.36 | 6.24 | 90.00 | 90.00 | 120.00 | 1.05 | 4.27 | 4.27 | 4.27 | 90.00 | 90.00 | 120.00 | 1.33 |
| mp-27853 | $Hg_3(TeBr)_2$ | $I2_13$ | 8.35 | 8.35 | 8.35 | 109.47 | 109.47 | 109.47 | 1.60 | 8.26 | 8.26 | 8.26 | 109.47 | 109.47 | 109.47 | 1.68 |

TABLE S1: The spacegroup (SG), Materials Project material-id (mp-id), lattice constants ($a$, $b$, $c$ in Å, $\alpha$, $\beta$, $\gamma$ in °) and bandgaps ($E_g$) of all 52 materials considered in this study. We have compared the lattice parameters and bandgaps (computed using DFT with the vdW-optB88 functional) obtained from our calculation with the values reported in the Materials Project database. The Materials Project employs DFT with PBE+U approximation which does not account for van der Waals effects that are prominent in layered materials.

## II. EXCITON BINDING ENERGY, OPTICAL GAP, AND QUASIPARTICLE GAPS FROM $G_0W_0$-BSE AND $GW_0$-BSE CALCULATIONS

| mp-id | Formula | $E_g^{PBE}$ | $E_g^{HSE}$ | $G_0W_0$-BSE | | | | $GW_0$-BSE | | | |
|---|---|---|---|---|---|---|---|---|---|---|---|
| | | | | OPG | QPGD | QPG | EBE | OPG | QPGD | QPG | EBE |
| mp-2657 | $TiO_2$ | 1.83 | 3.20 (D) | 3.07 | 3.28 | 3.28 | 0.21 | 3.91 | 4.27 | 4.26 | 0.35 |
| mp-34688 | $TiO_2$ | 2.22 | 3.50 (I) | 3.46 | 4.10 | 3.73 | 0.27 | 4.32 | 5.03 | 4.74 | 0.42 |
| mp-390 | $TiO_2$ | 2.07 | 3.50 (I) | 3.31 | 3.93 | 3.56 | 0.25 | 4.32 | 5.03 | 4.74 | 0.42 |
| mp-5229 | $SrTiO_3$ | 1.94 | 3.20 (I) | 3.24 | 3.80 | 3.48 | 0.24 | 4.21 | 4.86 | 4.57 | 0.37 |
| mp-4170 | $NaTaO_3$ | 2.46 | 3.10 (I) | 3.41 | 4.54 | 3.75 | 0.33 | 4.05 | 5.33 | 4.58 | 0.53 |
| mp-556489 | $Ta_2SnO_6$ | 2.10 | 3.10 (I) | 3.16 | 3.44 | 3.43 | 0.27 | 4.05 | 5.33 | 4.58 | 0.53 |
| mp-20194 | $CeO_2$ | 2.19 | 3.50 (I) | 3.58 | 4.08 | 3.98 | 0.40 | 5.76 | 6.83 | 6.55 | 0.79 |
| mp-36734 | $CeThO_4$ | 2.02 | 3.20 (I) | 3.42 | 3.95 | 3.86 | 0.45 | 5.73 | 6.97 | 6.68 | 0.95 |
| mp-8789 | $Ca_4As_2O$ | 1.29 | 2.00 (I) | 2.17 | 2.69 | 2.36 | 0.19 | 2.65 | 3.26 | 2.92 | 0.27 |
| mp-2172 | AlAs | 1.62 | 2.10 (I) | 2.04 | 2.77 | 2.18 | 0.13 | 2.26 | 3.04 | 2.43 | 0.16 |
| mp-8881 | AlAs | 1.82 | 2.40 (I) | 2.34 | 2.51 | 2.49 | 0.15 | 2.56 | 2.76 | 2.74 | 0.18 |
| mp-1863 | SiAs | 1.27 | 2.10 (I) | 1.40 | 1.62 | 1.52 | 0.13 | 1.52 | 1.77 | 1.67 | 0.15 |
| mp-27776 | $Cd_2AsCl_2$ | 1.06 | 1.80 (I) | 1.96 | 2.38 | 2.23 | 0.27 | 1.52 | 1.77 | 1.67 | 0.15 |
| mp-1009087 | $BeSiAs_2$ | 1.09 | 1.70 (D) | 1.54 | 1.66 | 1.66 | 0.12 | 1.73 | 1.87 | 1.87 | 0.15 |
| mp-1016197 | $MgSiAs_2$ | 1.39 | 1.90 (D) | 1.78 | 1.92 | 1.92 | 0.14 | 1.99 | 2.16 | 2.16 | 0.17 |
| mp-12558 | LiMgAs | 1.55 | 2.00 (I) | 2.16 | 2.72 | 2.33 | 0.17 | 2.44 | 3.06 | 2.66 | 0.21 |
| mp-961685 | NaCaAs | 1.83 | 2.20 (I) | 2.35 | 2.61 | 2.57 | 0.22 | 2.81 | 3.13 | 3.09 | 0.29 |
| mp-2624 | AlSb | 1.30 | 1.80 (I) | 1.71 | 2.45 | 1.83 | 0.11 | 1.89 | 2.66 | 2.02 | 0.14 |
| mp-9274 | $Rb_3Sb_2Au_3$ | 1.13 | 1.70 (D) | 1.64 | 2.13 | 1.86 | 0.23 | 1.89 | 2.66 | 2.02 | 0.14 |
| mp-1634 | $MoSe_2$ | 0.97 | 1.90 (D) | 1.08 | 1.89 | 1.22 | 0.14 | 1.14 | 1.99 | 1.30 | 0.16 |
| mp-1018807 | $MoSe_2$ | 0.95 | 1.90 (I) | 1.06 | 1.94 | 1.20 | 0.15 | 1.12 | 2.04 | 1.28 | 0.17 |
| mp-7581 | $MoSe_2$ | 1.07 | 1.90 (I) | 1.19 | 1.82 | 1.39 | 0.21 | 1.25 | 1.91 | 1.48 | 0.23 |
| mp-1821 | $WSe_2$ | 1.06 | 1.90 (I) | 1.18 | 2.15 | 1.33 | 0.15 | 1.25 | 2.24 | 1.41 | 0.17 |
| mp-1190 | ZnSe | 1.26 | 2.30 (D) | 2.30 | 2.49 | 2.49 | 0.19 | 2.65 | 2.89 | 2.89 | 0.23 |
| mp-15776 | $Zn(GaSe_2)_2$ | 1.43 | 2.30 (D) | 2.49 | 2.68 | 2.68 | 0.19 | 2.79 | 3.02 | 3.02 | 0.23 |
| mp-574620 | $CsYZnSe_3$ | 1.94 | 3.10 (D) | 3.36 | 3.68 | 3.68 | 0.32 | 2.79 | 3.02 | 3.02 | 0.23 |
| mp-510283 | $CsGaSe_3$ | 1.66 | 2.80 (I) | 2.43 | 3.06 | 3.02 | 0.59 | 2.77 | 3.64 | 3.60 | 0.83 |
| mp-1943 | GaSe | 0.56 | 2.10 (I) | 1.39 | 1.55 | 1.55 | 0.16 | 1.62 | 1.81 | 1.81 | 0.19 |
| mp-11342 | GaSe | 0.72 | 2.10 (I) | 1.67 | 1.82 | 1.82 | 0.16 | 1.88 | 2.07 | 2.07 | 0.19 |
| mp-1340 | $Ga_2Se_3$ | 0.17 | 1.90 (D) | 1.90 | 2.07 | 2.07 | 0.18 | 2.20 | 2.42 | 2.42 | 0.22 |
| mp-28423 | $Ga_2TeSe_2$ | 1.58 | 2.50 (D) | 2.53 | 2.74 | 2.72 | 0.19 | 2.85 | 3.10 | 3.08 | 0.23 |
| mp-567386 | $Cs_2Cd_3Te_4$ | 1.61 | 2.30 (D) | 2.39 | 2.73 | 2.73 | 0.34 | 2.59 | 2.99 | 2.99 | 0.40 |
| mp-12491 | $CsLaCdTe_3$ | 1.62 | 2.40 (D) | 2.34 | 2.56 | 2.56 | 0.23 | 2.59 | 2.99 | 2.99 | 0.40 |
| mp-20782 | $LiInTe_2$ | 1.40 | 2.10 (D) | 2.22 | 2.40 | 2.40 | 0.18 | 2.50 | 2.73 | 2.73 | 0.22 |
| mp-22255 | $RbInTe_2$ | 1.01 | 1.80 (I) | 1.92 | 2.58 | 2.21 | 0.28 | 2.19 | 2.97 | 2.55 | 0.36 |
| mp-35663 | $Sr(InTe_2)_2$ | 0.88 | 1.70 (I) | 1.71 | 2.34 | 1.89 | 0.18 | 1.93 | 2.63 | 2.15 | 0.22 |
| mp-9008 | RbTeAu | 1.05 | 1.70 (D) | 1.82 | 2.07 | 2.07 | 0.24 | 1.93 | 2.63 | 2.15 | 0.22 |
| mp-571195 | ZnTe | 0.92 | 2.00 (D) | 1.85 | 2.02 | 2.02 | 0.16 | 2.08 | 2.28 | 2.28 | 0.20 |
| mp-8884 | ZnTe | 1.38 | 2.10 (D) | 2.48 | 2.65 | 2.65 | 0.17 | 2.76 | 2.96 | 2.96 | 0.20 |
| mp-2176 | ZnTe | 1.16 | 2.10 (D) | 2.22 | 2.39 | 2.39 | 0.17 | 2.49 | 2.69 | 2.69 | 0.20 |
| mp-15777 | $Zn(GaTe_2)_2$ | 0.68 | 1.80 (I) | 1.82 | 1.98 | 1.98 | 0.16 | 2.04 | 2.23 | 2.23 | 0.19 |
| mp-13949 | $Cd(GaTe_2)_2$ | 1.01 | 1.80 (D) | 1.91 | 2.05 | 2.05 | 0.15 | 2.04 | 2.23 | 2.23 | 0.19 |
| mp-542812 | GaTe | 1.04 | 1.70 (D) | 1.44 | 1.57 | 1.57 | 0.13 | 1.59 | 1.76 | 1.76 | 0.16 |
| mp-1779 | YbTe | 1.54 | 2.10 (I) | 2.36 | 3.65 | 2.57 | 0.22 | 2.75 | 4.18 | 3.04 | 0.29 |
| mp-27449 | GaTeCl | 2.04 | 3.00 (D) | 2.99 | 3.27 | 3.24 | 0.25 | 3.31 | 3.65 | 3.62 | 0.31 |
| mp-29236 | InTeBr | 1.51 | 2.60 (D) | 2.33 | 2.54 | 2.54 | 0.21 | 2.65 | 2.91 | 2.91 | 0.27 |
| mp-33723 | BiTeBr | 1.05 | 1.80 (I) | 1.56 | 1.71 | 1.71 | 0.15 | 1.72 | 1.89 | 1.89 | 0.17 |
| mp-27853 | $Hg_3(TeBr)_2$ | 1.60 | 2.50 (D) | 2.51 | 2.86 | 2.74 | 0.23 | 2.79 | 3.19 | 3.06 | 0.28 |

TABLE S2: Computed optical gap (OPG), direct (QPGD) and indirect (QPG) quasiparticle gaps (in eV) obtained from $G_0W_0$-BSE as well as $GW_0$-BSE calculations for all the materials considered in this study. The table also lists the DFT bandgaps obtained by using both PBE, $E_g^{PBE}$, and HSE06, $E_g^{HSE}$, exchange-correlation functional. The $E_g^{HSE}$ data is taken from Singh et al.'s work. [1]

## III. COMPUTED $\alpha_{\text{int}}$ FOR ALL THREE POLARIZATION AXIS ,$\alpha_{\text{int}}^{\text{avg}}$, AND $\alpha_{\text{int}}^{\text{aniso}}$ IN THE VISIBLE (1.7-3.5 EV) AS WELL AS UV RANGE (3.5-4.2 EV)

| mp-id | Formula | $\alpha_{\text{int}}^{x}$ | $\alpha_{\text{int}}^{y}$ | $\alpha_{\text{int}}^{z}$ | $\alpha_{\text{int}}^{\text{avg}}$ | $\alpha_{\text{int}}^{\text{aniso}}$ |
|---|---|---|---|---|---|---|
| mp-2657 | $TiO_2$ | 0.88 | 0.68 | 0.68 | 0.75 | 0.77 |
| mp-34688 | $TiO_2$ | 0.28 | 0.28 | 0.29 | 0.28 | 0.96 |
| mp-390 | $TiO_2$ | 0.52 | 0.51 | 0.37 | 0.47 | 0.72 |
| mp-5229 | $SrTiO_3$ | 0.54 | 0.54 | 0.53 | 0.54 | 1.00 |
| mp-4170 | $NaTaO_3$ | 0.21 | 0.21 | 0.21 | 0.21 | 1.00 |
| mp-556489 | $Ta_2SnO_6$ | 0.39 | 0.52 | 1.16 | 0.69 | 0.33 |
| mp-20194 | $CeO_2$ | 0.59 | 0.59 | 0.59 | 0.59 | 1.00 |
| mp-36734 | $CeThO_4$ | 0.00 | 0.00 | 0.00 | 0.00 | 0.00 |
| mp-8789 | $Ca_4As_2O$ | 4.00 | 3.96 | 1.77 | 3.24 | 0.44 |
| mp-2172 | AlAs | 2.77 | 2.77 | 2.77 | 2.77 | 1.00 |
| mp-8881 | AlAs | 2.67 | 2.67 | 2.18 | 2.51 | 0.82 |
| mp-1863 | SiAs | 7.30 | 7.21 | 5.87 | 6.79 | 0.80 |
| mp-27776 | $Cd_2AsCl_2$ | 2.72 | 4.02 | 0.95 | 2.57 | 0.24 |
| mp-1009087 | $BeSiAs_2$ | 2.85 | 2.85 | 3.08 | 2.92 | 0.92 |
| mp-1016197 | $MgSiAs_2$ | 6.68 | 6.68 | 8.53 | 7.30 | 0.78 |
| mp-12558 | LiMgAs | 2.19 | 2.19 | 2.19 | 2.19 | 1.00 |
| mp-961685 | NaCaAs | 4.37 | 4.37 | 4.37 | 4.37 | 1.00 |
| mp-2624 | AlSb | 8.00 | 8.00 | 8.00 | 8.00 | 1.00 |
| mp-9274 | $Rb_3Sb_2Au_3$ | 13.57 | 14.11 | 9.26 | 12.31 | 0.66 |
| mp-1634 | $MoSe_2$ | 17.51 | 17.50 | 5.20 | 13.40 | 0.30 |
| mp-1018807 | $MoSe_2$ | 17.97 | 17.99 | 5.68 | 13.88 | 0.32 |
| mp-7581 | $MoSe_2$ | 16.80 | 17.15 | 6.29 | 13.41 | 0.37 |
| mp-1821 | $WSe_2$ | 14.38 | 14.37 | 4.47 | 11.07 | 0.31 |
| mp-1190 | ZnSe | 2.12 | 2.11 | 2.12 | 2.12 | 1.00 |
| mp-15776 | $Zn(GaSe_2)_2$ | 2.11 | 2.11 | 2.10 | 2.11 | 0.99 |
| mp-574620 | $CsYZnSe_3$ | 0.75 | 0.15 | 0.46 | 0.45 | 0.21 |
| mp-510283 | $CsGaSe_3$ | 0.00 | 0.00 | 0.00 | 0.00 | 0.00 |
| mp-1943 | GaSe | 2.13 | 2.13 | 2.07 | 2.11 | 0.97 |
| mp-11342 | GaSe | 2.30 | 2.28 | 2.96 | 2.51 | 0.77 |
| mp-1340 | $Ga_2Se_3$ | 3.39 | 4.84 | 3.81 | 4.01 | 0.70 |
| mp-28423 | $Ga_2TeSe_2$ | 3.12 | 2.89 | 2.55 | 2.85 | 0.82 |
| mp-567386 | $Cs_2Cd_3Te_4$ | 0.00 | 0.00 | 0.00 | 0.00 | 0.00 |
| mp-12491 | $CsLaCdTe_3$ | 2.52 | 1.06 | 0.82 | 1.47 | 0.33 |
| mp-20782 | $LiInTe_2$ | 5.49 | 5.61 | 6.34 | 5.81 | 0.87 |
| mp-22255 | $RbInTe_2$ | 5.43 | 8.50 | 6.28 | 6.73 | 0.64 |
| mp-35663 | $Sr(InTe_2)_2$ | 8.13 | 11.48 | 6.10 | 8.57 | 0.53 |
| mp-9008 | RbTeAu | 0.32 | 9.39 | 1.99 | 3.90 | 0.03 |
| mp-571195 | ZnTe | 4.93 | 4.93 | 6.67 | 5.51 | 0.74 |
| mp-8884 | ZnTe | 2.36 | 2.36 | 2.24 | 2.32 | 0.95 |
| mp-2176 | ZnTe | 3.41 | 3.41 | 3.41 | 3.41 | 1.00 |
| mp-15777 | $Zn(GaTe_2)_2$ | 6.97 | 7.02 | 7.21 | 7.07 | 0.97 |
| mp-13949 | $Cd(GaTe_2)_2$ | 8.05 | 8.10 | 8.39 | 8.18 | 0.96 |
| mp-542812 | GaTe | 9.09 | 9.56 | 9.61 | 9.42 | 0.95 |
| mp-1779 | YbTe | 1.18 | 1.18 | 1.18 | 1.18 | 1.00 |
| mp-27449 | GaTeCl | 4.27 | 1.46 | 0.33 | 2.02 | 0.08 |
| mp-29236 | InTeBr | 5.86 | 6.42 | 4.53 | 5.61 | 0.71 |
| mp-33723 | BiTeBr | 14.26 | 14.25 | 3.75 | 10.75 | 0.26 |
| mp-27853 | $Hg_3(TeBr)_2$ | 4.04 | 4.08 | 4.06 | 4.06 | 0.99 |

TABLE S3: Computed $\alpha_{\text{int}}$ (in $10^4$ cm$^{-1}$ eV) for all three polarization axis, $\alpha_{\text{int}}^{\text{avg}}$ (in $10^4$ cm$^{-1}$ eV), and $\alpha_{\text{int}}^{\text{aniso}}$ in the visible range (1.7-3.5 eV)

| mp-id | Formula | $\alpha_{\text{int}}^{x}$ | $\alpha_{\text{int}}^{y}$ | $\alpha_{\text{int}}^{z}$ | $\alpha_{\text{int}}^{\text{avg}}$ | $\alpha_{\text{int}}^{\text{aniso}}$ |
|---|---|---|---|---|---|---|
| mp-2657 | $TiO_2$ | 8.95 | 7.45 | 7.45 | 7.95 | 0.83 |
| mp-34688 | $TiO_2$ | 2.36 | 2.36 | 3.15 | 2.62 | 0.75 |
| mp-390 | $TiO_2$ | 4.08 | 4.02 | 2.89 | 3.66 | 0.71 |
| mp-5229 | $SrTiO_3$ | 4.15 | 4.15 | 4.15 | 4.15 | 1.00 |
| mp-4170 | NaTaO3 | 1.23 | 1.23 | 1.23 | 1.23 | 1.00 |
| mp-556489 | $Ta_2SnO_6$ | 2.31 | 3.63 | 4.15 | 3.36 | 0.56 |
| mp-20194 | $CeO_2$ | 7.70 | 7.70 | 7.70 | 7.70 | 1.00 |
| mp-36734 | $CeThO_4$ | 0.00 | 0.00 | 0.00 | 0.00 | 0.00 |
| mp-8789 | $Ca_4As_2O$ | 8.33 | 8.32 | 7.82 | 8.16 | 0.94 |
| mp-2172 | AlAs | 10.69 | 10.68 | 10.68 | 10.68 | 1.00 |
| mp-8881 | AlAs | 10.43 | 10.43 | 13.93 | 11.60 | 0.75 |
| mp-1863 | SiAs | 17.71 | 14.48 | 14.17 | 15.45 | 0.80 |
| mp-27776 | $Cd_2AsCl_2$ | 4.59 | 5.50 | 4.47 | 4.85 | 0.81 |
| mp-1009087 | $BeSiAs_2$ | 11.04 | 11.04 | 11.69 | 11.26 | 0.94 |
| mp-1016197 | $MgSiAs_2$ | 12.62 | 12.62 | 13.84 | 13.03 | 0.91 |
| mp-12558 | LiMgAs | 9.46 | 9.45 | 9.46 | 9.46 | 1.00 |
| mp-961685 | NaCaAs | 6.72 | 6.71 | 6.72 | 6.72 | 1.00 |
| mp-2624 | AlSb | 19.24 | 19.24 | 19.24 | 19.24 | 1.00 |
| mp-9274 | $Rb_3Sb_2Au_3$ | 13.67 | 14.04 | 11.10 | 12.94 | 0.79 |
| mp-1634 | $MoSe_2$ | 16.44 | 16.43 | 4.66 | 12.51 | 0.28 |
| mp-1018807 | $MoSe_2$ | 16.73 | 16.73 | 4.31 | 12.59 | 0.26 |
| mp-7581 | $MoSe_2$ | 14.84 | 15.16 | 5.27 | 11.76 | 0.35 |
| mp-1821 | $WSe_2$ | 14.56 | 14.56 | 4.79 | 11.30 | 0.33 |
| mp-1190 | ZnSe | 3.99 | 3.98 | 3.99 | 3.99 | 1.00 |
| mp-15776 | $Zn(GaSe_2)_2$ | 5.88 | 5.92 | 6.15 | 5.98 | 0.96 |
| mp-574620 | $CsYZnSe_3$ | 4.39 | 1.17 | 2.23 | 2.60 | 0.27 |
| mp-510283 | $CsGaSe_3$ | 0.00 | 0.00 | 0.00 | 0.00 | 0.00 |
| mp-1943 | GaSe | 6.61 | 6.61 | 5.56 | 6.26 | 0.84 |
| mp-11342 | GaSe | 6.38 | 6.44 | 4.18 | 5.66 | 0.65 |
| mp-1340 | $Ga2Se_3$ | 7.21 | 7.19 | 7.20 | 7.20 | 1.00 |
| mp-28423 | $Ga_2TeSe_2$ | 7.29 | 7.02 | 6.63 | 6.98 | 0.91 |
| mp-567386 | $Cs_2Cd_3Te_4$ | 0.00 | 0.00 | 0.00 | 0.00 | 0.00 |
| mp-12491 | $CsLaCdTe_3$ | 3.63 | 1.71 | 1.59 | 2.31 | 0.44 |
| mp-20782 | $LiInTe_2$ | 8.37 | 8.52 | 9.39 | 8.76 | 0.89 |
| mp-22255 | $RbInTe_2$ | 6.15 | 10.57 | 7.18 | 7.97 | 0.58 |
| mp-35663 | $Sr(InTe_2)_2$ | 9.29 | 13.01 | 6.86 | 9.72 | 0.53 |
| mp-9008 | RbTeAu | 0.93 | 12.60 | 9.44 | 7.66 | 0.07 |
| mp-571195 | ZnTe | 12.13 | 12.13 | 13.41 | 12.56 | 0.90 |
| mp-8884 | ZnTe | 8.10 | 8.10 | 9.10 | 8.43 | 0.89 |
| mp-8884 | ZnTe | 6.84 | 6.84 | 7.33 | 7.00 | 0.93 |
| mp-2176 | ZnTe | 8.86 | 8.86 | 8.86 | 8.86 | 1.00 |
| mp-15777 | $Zn(GaTe_2)_2$ | 10.61 | 10.66 | 10.94 | 10.74 | 0.97 |
| mp-13949 | $Cd(GaTe_2)_2$ | 11.46 | 11.47 | 11.89 | 11.61 | 0.96 |
| mp-542812 | GaTe | 16.65 | 12.10 | 13.48 | 14.08 | 0.73 |
| mp-1779 | YbTe | 5.85 | 5.85 | 5.85 | 5.85 | 1.00 |
| mp-27449 | GaTeCl | 15.21 | 7.17 | 1.58 | 7.98 | 0.10 |
| mp-29236 | InTeBr | 8.80 | 12.08 | 7.53 | 9.47 | 0.62 |
| mp-33723 | BiTeBr | 21.87 | 21.86 | 6.97 | 16.90 | 0.32 |
| mp-27853 | $Hg_3(TeBr)_2$ | 10.02 | 10.14 | 10.08 | 10.08 | 0.99 |

TABLE S4: Computed $\alpha_{\text{int}}$ (in $10^4$ cm$^{-1}$ eV) for all three polarization axis, $\alpha_{\text{int}}^{\text{avg}}$ (in $10^4$ cm$^{-1}$ eV), and $\alpha_{\text{int}}^{\text{aniso}}$ in the UV Range (3.5-4.2 eV)

## IV. COMPARISON OF WANNIER MOTT (WM) AND BSE EXCITON BINDING ENERGIES

| mp-id | Formula | $EBE_{BSE}$(eV) | $EBE_{WM}$(eV) |
|---|---|---|---|
| mp-34688 | $TiO_2$ | 0.27 | 0.09 |
| mp-390 | $TiO_2$ | 0.25 | 0.10 |
| mp-5229 | $SrTiO_3$ | 0.24 | 0.09 |
| mp-20194 | $CeO_2$ | 0.40 | 0.13 |
| mp-36734 | $CeThO_4$ | 0.45 | 0.23 |
| mp-8789 | $Ca_4As_2O$ | 0.19 | 0.02 |
| mp-2172 | AlAs | 0.13 | 0.01 |
| mp-8881 | AlAs | 0.15 | 0.01 |
| mp-1863 | SiAs | 0.13 | 0.01 |
| mp-1863 | SiAs | 0.13 | 0.02 |
| mp-27776 | $Cd_2AsCl_2$ | 0.27 | 0.07 |
| mp-27776 | $Cd_2AsCl_2$ | 0.27 | 0.07 |
| mp-1009087 | $BeSiAs_2$ | 0.12 | 0.01 |
| mp-1016197 | $MgSiAs_2$ | 0.14 | 0.01 |
| mp-12558 | LiMgAs | 0.17 | 0.01 |
| mp-961685 | NaCaAs | 0.22 | 0.04 |
| mp-2624 | AlSb | 0.11 | 0.00 |
| mp-1634 | $MoSe_2$ | 0.14 | 0.02 |
| mp-1018807 | $MoSe_2$ | 0.15 | 0.02 |
| mp-7581 | $MoSe_2$ | 0.21 | 0.03 |
| mp-1821 | $WSe_2$ | 0.15 | 0.02 |
| mp-1190 | ZnSe | 0.19 | 0.01 |
| mp-574620 | $CsYZnSe_3$ | 0.32 | 0.04 |
| mp-1943 | GaSe | 0.16 | 0.02 |
| mp-11342 | GaSe | 0.16 | 0.02 |
| mp-1340 | $Ga_2Se_3$ | 0.18 | 0.01 |
| mp-28423 | $Ga_2TeSe_2$ | 0.19 | 0.02 |
| mp-12491 | $CsLaCdTe_3$ | 0.23 | 0.03 |
| mp-20782 | $LiInTe_2$ | 0.18 | 0.02 |
| mp-22255 | $RbInTe_2$ | 0.28 | 0.06 |
| mp-35663 | $Sr(InTe_2)_2$ | 0.18 | 0.01 |
| mp-9008 | RbTeAu | 0.24 | 0.11 |
| mp-571195 | ZnTe | 0.16 | 0.00 |
| mp-8884 | ZnTe | 0.17 | 0.00 |
| mp-2176 | ZnTe | 0.17 | 0.00 |
| mp-15777 | $Zn(GaTe_2)_2$ | 0.16 | 0.00 |
| mp-13949 | $Cd(GaTe_2)_2$ | 0.15 | 0.00 |
| mp-542812 | GaTe | 0.13 | 0.02 |
| mp-1779 | YbTe | 0.22 | 0.02 |
| mp-29236 | InTeBr | 0.21 | 0.05 |
| mp-29236 | InTeBr | 0.21 | 0.04 |
| mp-33723 | BiTeBr | 0.15 | 0.01 |
| mp-27853 | $Hg_3(TeBr)_2$ | 0.23 | 0.04 |

TABLE S5: The Materials Project material-id (mp-id), exciton binding energies computed using Wannier Mott model, $EBE_{WM}$ and BSE calculations, $EBE_{BSE}$.

## V. ADDITIONAL PARAMETERS USED IN THE $G_0W_0$-BSE CALCULATION

| mp-id | Formula | $N_{\mathrm{bands}}^{\mathrm{GW}}$ | $k$-grid | $N_{\mathrm{bands}}^{\mathrm{occ}}$ | $E_{\mathrm{VBE}}^{\mathrm{max}}$ (eV) | $E_{\mathrm{CBE}}^{\mathrm{max}}$ (eV) |
|---|---|---|---|---|---|---|
| mp-2657 | $TiO_2$ | 480 | 12×7×7 | 24 | 8.84 | 9.78 |
| mp-34688 | $TiO_2$ | 280 | 7×7×6 | 24 | 9.78 | 9.83 |
| mp-390 | $TiO_2$ | 480 | 10×10×7 | 24 | 9.43 | 9.58 |
| mp-5229 | $SrTiO_3$ | 480 | 9×9×9 | 20 | 22.71 | 12.06 |
| mp-4170 | $NaTaO_3$ | 280 | 7×7×7 | 20 | 25.17 | 17.31 |
| mp-556489 | $Ta_2SnO_6$ | 480 | 7×6×4 | 76 | 6.55 | 6.78 |
| mp-20194 | $CeO_2$ | 720 | 10×10×10 | 12 | 22.36 | 10.81 |
| mp-36734 | $CeThO_4$ | 280 | 12×6×7 | 24 | 8.11 | 9.62 |
| mp-8789 | $Ca_4As_2O$ | 720 | 8×8×4 | 28 | 12.96 | 7.94 |
| mp-2172 | AlAs | 480 | 10×10×10 | 4 | 15.30 | 19.92 |
| mp-8881 | AlAs | 720 | 9×9×5 | 8 | 15.20 | 12.59 |
| mp-1863 | SiAs | 720 | 10×4×3 | 27 | 5.77 | 6.39 |
| mp-27776 | $Cd_2AsCl_2$ | 480 | 4×4×4 | 118 | 6.10 | 6.13 |
| mp-1009087 | $BeSiAs_2$ | 720 | 7×7×6 | 18 | 8.70 | 9.01 |
| mp-1016197 | $MgSiAs_2$ | 960 | 6×6×5 | 24 | 7.31 | 7.22 |
| mp-12558 | LiMgAs | 720 | 9×9×9 | 9 | 87.54 | 16.88 |
| mp-961685 | NaCaAs | 720 | 8×8×8 | 12 | 31.34 | 12.17 |
| mp-2624 | AlSb | 720 | 9×9×9 | 9 | 34.46 | 17.04 |
| mp-9274 | $Rb_3Sb_2Au_3$ | 1200 | 5×5×5 | 57 | 6.51 | 7.31 |
| mp-1634 | $MoSe_2$ | 480 | 11×11×2 | 26 | 6.83 | 9.03 |
| mp-1018807 | $MoSe_2$ | 480 | 11×11×2 | 26 | 6.59 | 9.20 |
| mp-7581 | $MoSe_2$ | 480 | 9×9×9 | 13 | 37.92 | 13.85 |
| mp-1821 | $WSe_2$ | 720 | 11×11×2 | 26 | 7.77 | 8.63 |
| mp-1190 | ZnSe | 480 | 10×10×10 | 13 | 90.63 | 23.39 |
| mp-15776 | $Zn(GaSe_2)_2$ | 480 | 7×7×5 | 35 | 8.91 | 9.55 |
| mp-574620 | $CsYZnSe_3$ | 960 | 8×4×3 | 58 | 6.48 | 7.28 |
| mp-510283 | $CsGaSe_3$ | 280 | 4×3×2 | 80 | 4.86 | 5.69 |
| mp-1943 | GaSe | 480 | 10×10×2 | 38 | 7.68 | 8.63 |
| mp-11342 | GaSe | 480 | 7×7×7 | 19 | 19.94 | 13.00 |
| mp-1340 | $Ga_2Se_3$ | 480 | 5×5×5 | 44 | 6.62 | 7.17 |
| mp-28423 | $Ga_2TeSe_2$ | 480 | 5×5×5 | 44 | 6.32 | 6.82 |
| mp-567386 | $Cs_2Cd_3Te_4$ | 280 | 4×2×2 | 102 | 5.24 | 5.41 |
| mp-12491 | $CsLaCdTe_3$ | 720 | 7×4×3 | 58 | 6.56 | 7.49 |
| mp-20782 | $LiInTe_2$ | 480 | 6×6×5 | 28 | 6.17 | 7.58 |
| mp-22255 | $RbInTe_2$ | 480 | 5×5×5 | 34 | 5.95 | 7.17 |
| mp-35663 | $Sr(InTe_2)_2$ | 720 | 5×5×5 | 30 | 6.32 | 6.79 |
| mp-9008 | RbTeAu | 1200 | 7×6×5 | 34 | 8.13 | 9.32 |
| mp-571195 | ZnTe | 480 | 8×8×3 | 39 | 11.02 | 9.72 |
| mp-8884 | ZnTe | 480 | 9×9×5 | 26 | 12.16 | 12.85 |
| mp-2176 | ZnTe | 480 | 9×9×9 | 13 | 90.01 | 19.13 |
| mp-15777 | $Zn(GaTe_2)_2$ | 480 | 6×6×5 | 35 | 7.51 | 7.62 |
| mp-13949 | $Cd(GaTe_2)_2$ | 480 | 6×6×5 | 35 | 7.23 | 7.68 |
| mp-542812 | GaTe | 480 | 9×4×3 | 57 | 5.42 | 6.04 |
| mp-1779 | YbTe | 720 | 9×9×9 | 7 | 29.17 | 15.46 |
| mp-27449 | GaTeCl | 480 | 8×6×2 | 52 | 6.30 | 8.02 |
| mp-29236 | InTeBr | 480 | 5×4×4 | 52 | 5.25 | 6.56 |
| mp-33723 | BiTeBr | 480 | 8×8×6 | 15 | 29.24 | 14.39 |
| mp-27853 | $Hg_3(TeBr)_2$ | 1200 | 4×4×4 | 86 | 5.13 | 7.84 |

TABLE S6: The Materials Project material-id (mp-id), number of occupied bands ($N_{\mathrm{bands}}^{\mathrm{occ}}$), number of bands ($N_{\mathrm{bands}}^{\mathrm{GW}}$) and $k$-grid used in the GW-BSE calculations reported in this study.

## VI. ABSORPTION SPECTRA OBTAINED FROM $G_0W_0$-BSE CALCULATION

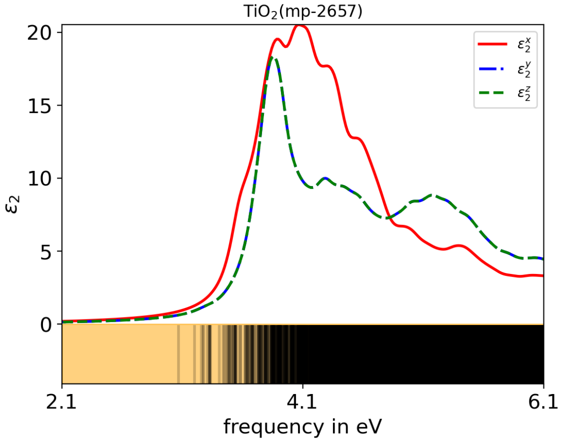

TiO$_2$(mp-2657)
$\varepsilon_2^x$
$\varepsilon_2^y$
$\varepsilon_2^z$
$\varepsilon_2$
frequency in eV


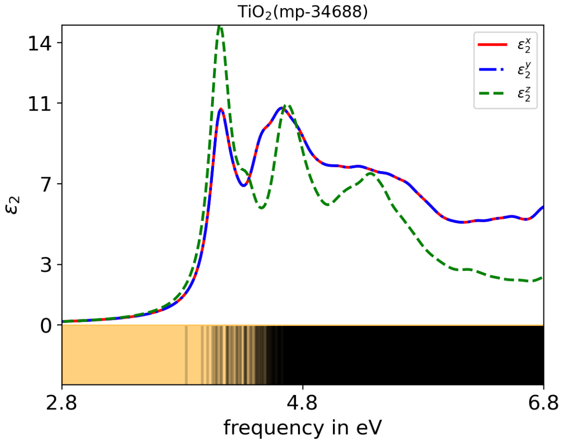

TiO$_2$(mp-34688)
$\varepsilon_2^x$
$\varepsilon_2^y$
$\varepsilon_2^z$
$\varepsilon_2$
frequency in eV


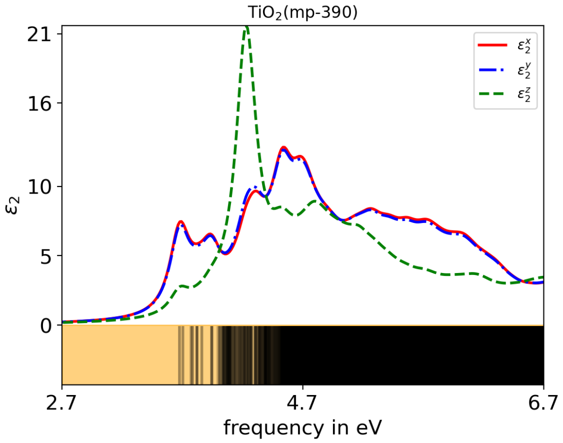

TiO$_2$(mp-390)
$\varepsilon_2^x$
$\varepsilon_2^y$
$\varepsilon_2^z$
$\varepsilon_2$
frequency in eV


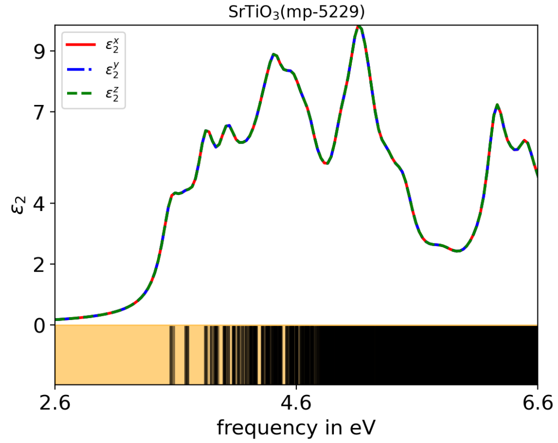

SrTiO$_3$(mp-5229)
$\varepsilon_2^x$
$\varepsilon_2^y$
$\varepsilon_2^z$
$\varepsilon_2$
frequency in eV

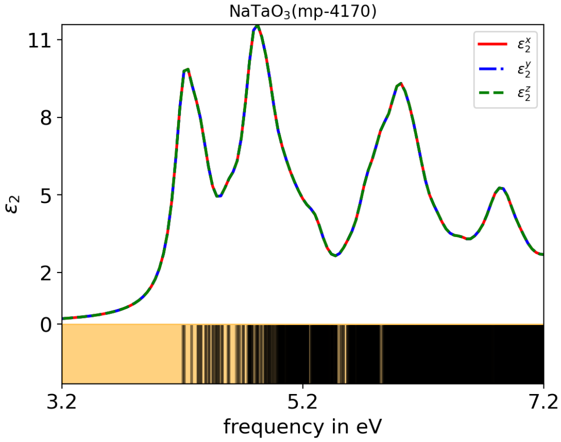
NaTaO$_3$(mp-4170)
$\varepsilon_2^x$
$\varepsilon_2^y$
$\varepsilon_2^z$
$\varepsilon_2$
11
8
5
2
0
3.2
5.2
7.2
frequency in eV

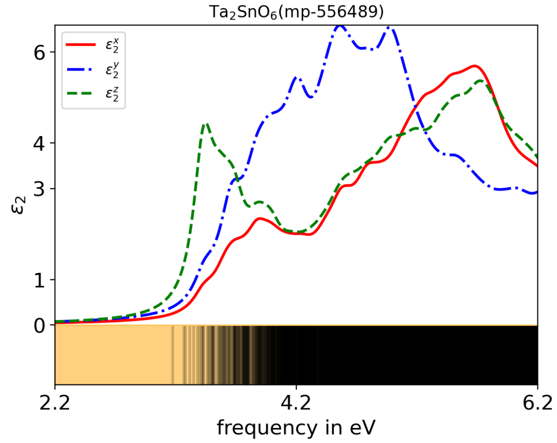
Ta$_2$SnO$_6$(mp-556489)
$\varepsilon_2^x$
$\varepsilon_2^y$
$\varepsilon_2^z$
$\varepsilon_2$
6
4
3
1
0
2.2
4.2
6.2
frequency in eV

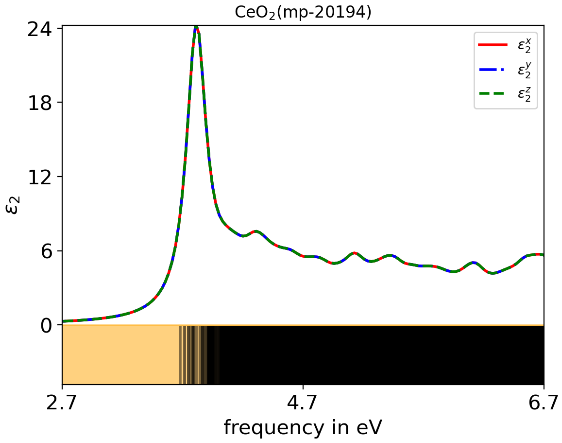
CeO$_2$(mp-20194)
$\varepsilon_2^x$
$\varepsilon_2^y$
$\varepsilon_2^z$
$\varepsilon_2$
24
18
12
6
0
2.7
4.7
6.7
frequency in eV

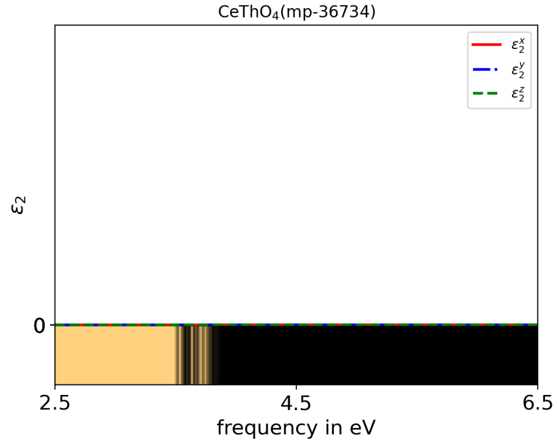
CeThO$_4$(mp-36734)
$\varepsilon_2^x$
$\varepsilon_2^y$
$\varepsilon_2^z$
$\varepsilon_2$
0
2.5
4.5
6.5
frequency in eV

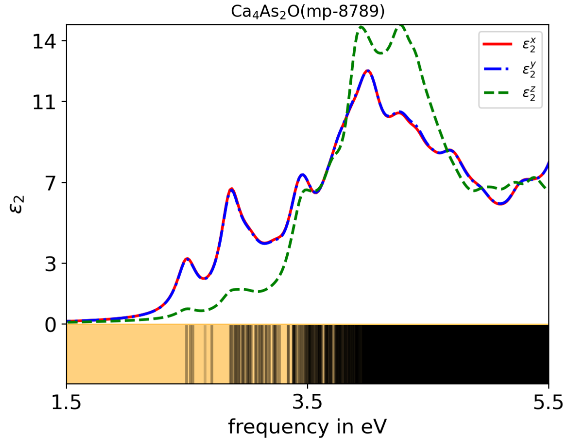

Ca$_4$As$_2$O(mp-8789)
$\varepsilon_2^x$
$\varepsilon_2^y$
$\varepsilon_2^z$
$\varepsilon_2$
14
11
7
3
0
1.5
3.5
5.5
frequency in eV


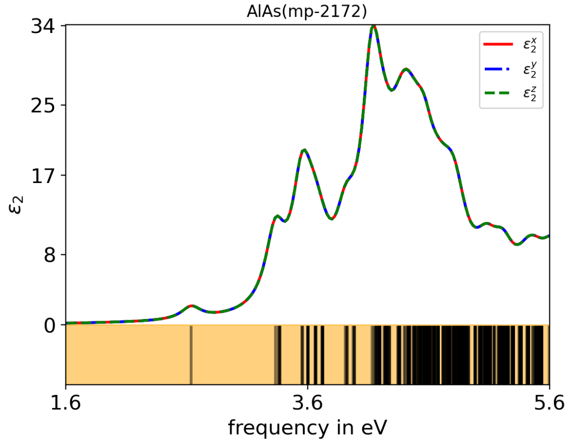

AlAs(mp-2172)
$\varepsilon_2^x$
$\varepsilon_2^y$
$\varepsilon_2^z$
$\varepsilon_2$
34
25
17
8
0
1.6
3.6
5.6
frequency in eV


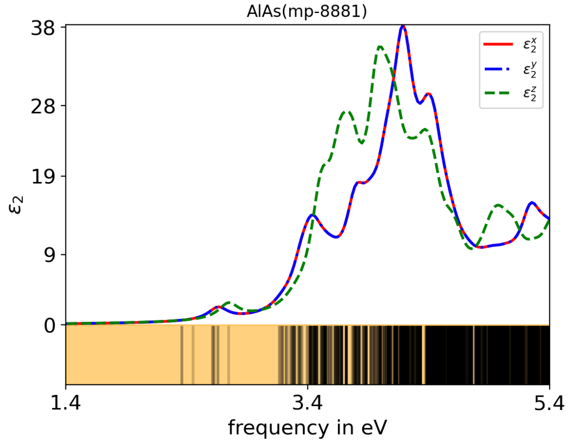

AlAs(mp-8881)
$\varepsilon_2^x$
$\varepsilon_2^y$
$\varepsilon_2^z$
$\varepsilon_2$
38
28
19
9
0
1.4
3.4
5.4
frequency in eV


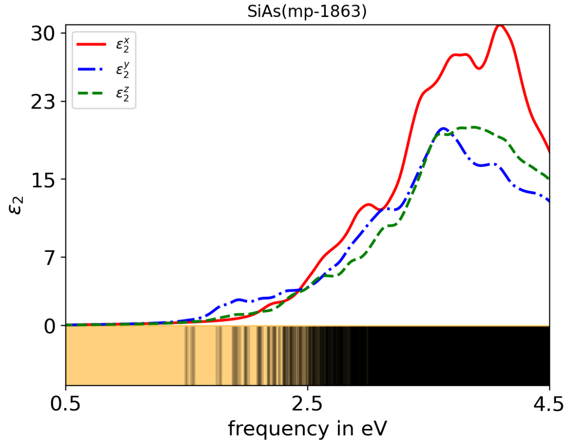

SiAs(mp-1863)
$\varepsilon_2^x$
$\varepsilon_2^y$
$\varepsilon_2^z$
$\varepsilon_2$
30
23
15
7
0
0.5
2.5
4.5
frequency in eV

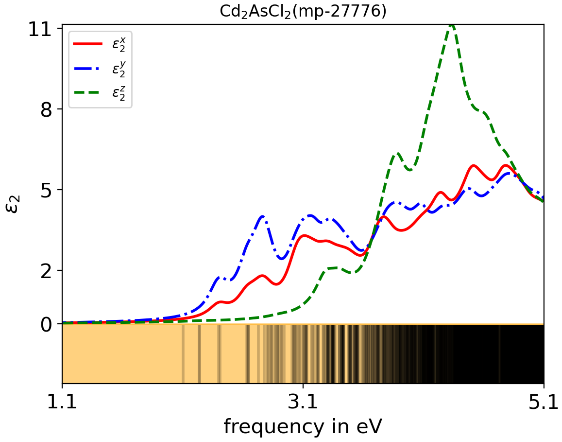
Cd$_2$AsCl$_2$(mp-27776)
$\varepsilon_2^x$
$\varepsilon_2^y$
$\varepsilon_2^z$
$\varepsilon_2$
0
2
5
8
11
1.1
3.1
5.1
frequency in eV

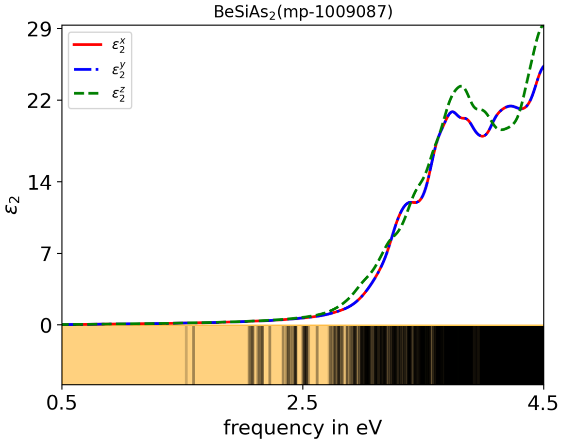
BeSiAs$_2$(mp-1009087)
$\varepsilon_2^x$
$\varepsilon_2^y$
$\varepsilon_2^z$
$\varepsilon_2$
0
7
14
22
29
0.5
2.5
4.5
frequency in eV

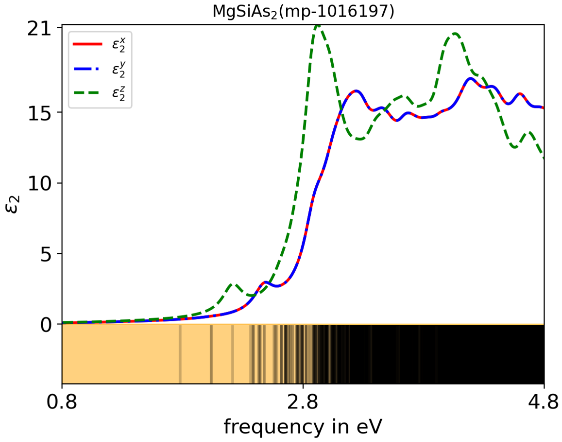
MgSiAs$_2$(mp-1016197)
$\varepsilon_2^x$
$\varepsilon_2^y$
$\varepsilon_2^z$
$\varepsilon_2$
0
5
10
15
21
0.8
2.8
4.8
frequency in eV

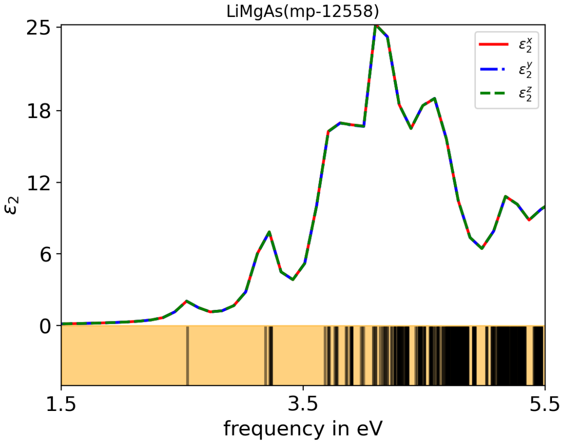
LiMgAs(mp-12558)
$\varepsilon_2^x$
$\varepsilon_2^y$
$\varepsilon_2^z$
$\varepsilon_2$
0
6
12
18
25
1.5
3.5
5.5
frequency in eV

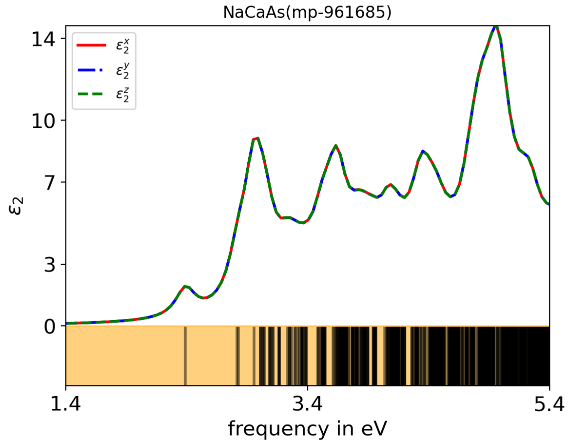
NaCaAs(mp-961685)
$\varepsilon_2^x$
$\varepsilon_2^y$
$\varepsilon_2^z$
14
10
7
3
0
$\varepsilon_2$
1.4
3.4
5.4
frequency in eV

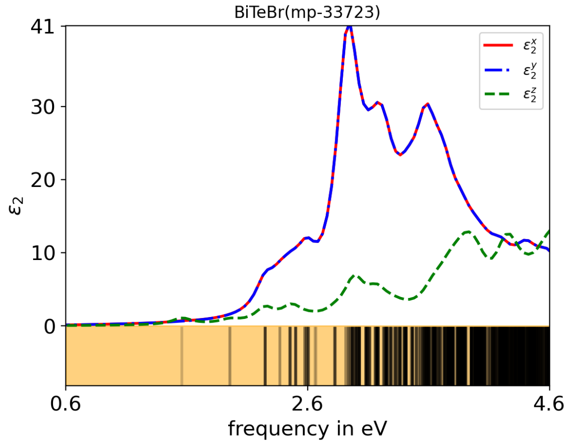
BiTeBr(mp-33723)
$\varepsilon_2^x$
$\varepsilon_2^y$
$\varepsilon_2^z$
41
30
20
10
0
$\varepsilon_2$
0.6
2.6
4.6
frequency in eV

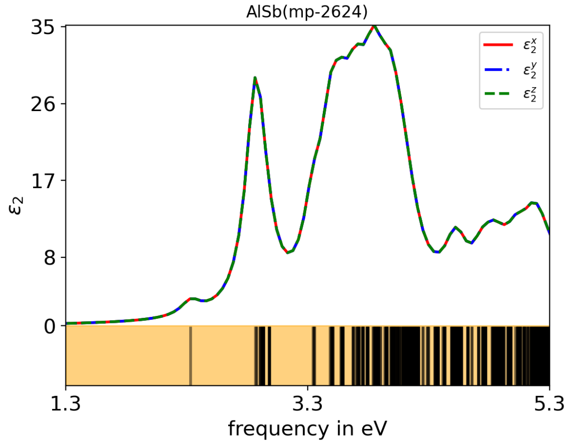
AlSb(mp-2624)
$\varepsilon_2^x$
$\varepsilon_2^y$
$\varepsilon_2^z$
35
26
17
8
0
$\varepsilon_2$
1.3
3.3
5.3
frequency in eV

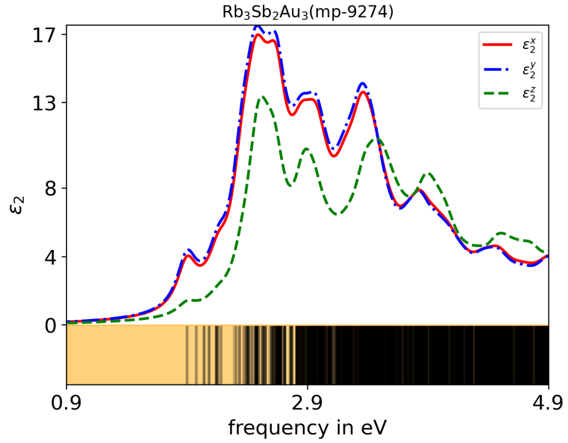
$Rb_3Sb_2Au_3$(mp-9274)
$\varepsilon_2^x$
$\varepsilon_2^y$
$\varepsilon_2^z$
17
13
8
4
0
$\varepsilon_2$
0.9
2.9
4.9
frequency in eV

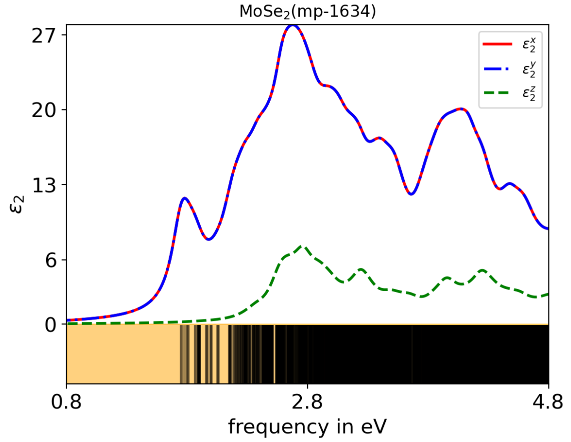
MoSe2(mp-1634)
ε2x
ε2y
ε2z
27
20
13
6
0
ε2
0.8
2.8
4.8
frequency in eV

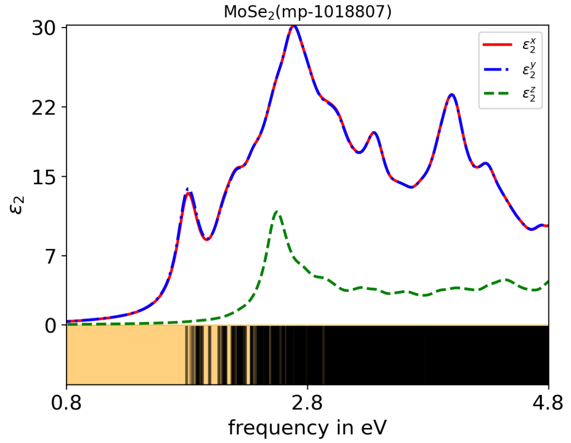
MoSe2(mp-1018807)
ε2x
ε2y
ε2z
30
22
15
7
0
ε2
0.8
2.8
4.8
frequency in eV

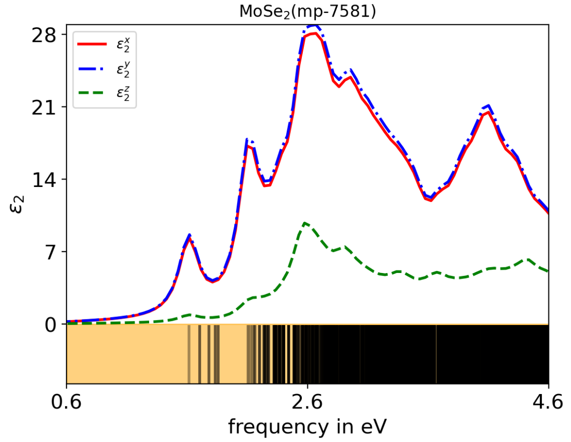
MoSe2(mp-7581)
ε2x
ε2y
ε2z
28
21
14
7
0
ε2
0.6
2.6
4.6
frequency in eV

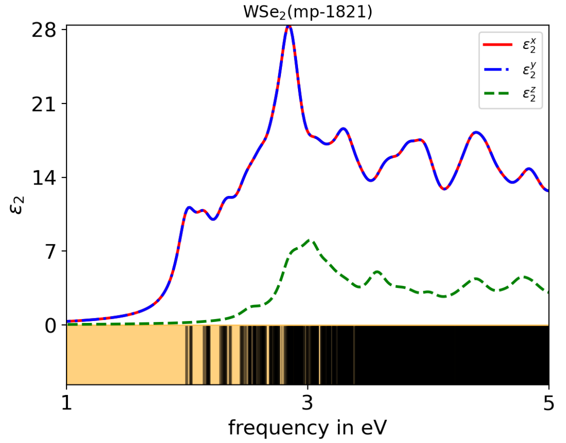
WSe2(mp-1821)
ε2x
ε2y
ε2z
28
21
14
7
0
ε2
1
3
5
frequency in eV

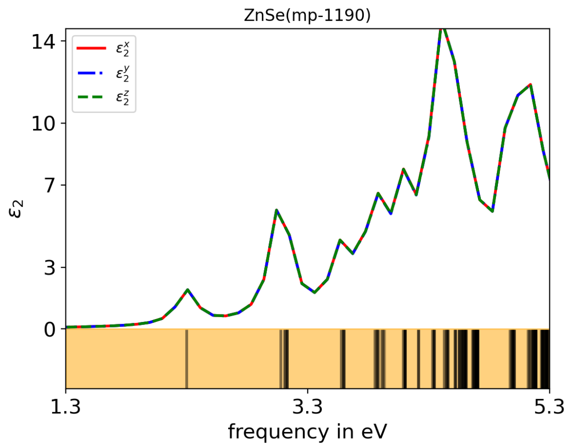
ZnSe(mp-1190)
$\varepsilon_2^x$
$\varepsilon_2^y$
$\varepsilon_2^z$
$\varepsilon_2$
frequency in eV

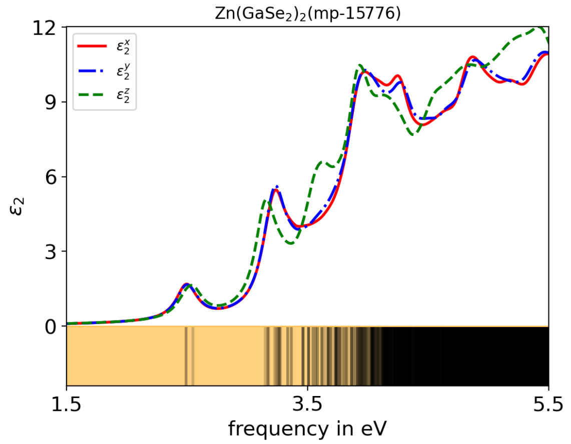
Zn(GaSe$_2$)$_2$(mp-15776)
$\varepsilon_2^x$
$\varepsilon_2^y$
$\varepsilon_2^z$
$\varepsilon_2$
frequency in eV

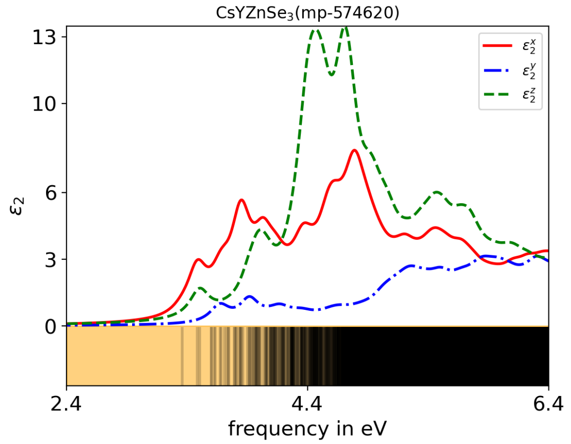
CsYZnSe$_3$(mp-574620)
$\varepsilon_2^x$
$\varepsilon_2^y$
$\varepsilon_2^z$
$\varepsilon_2$
frequency in eV

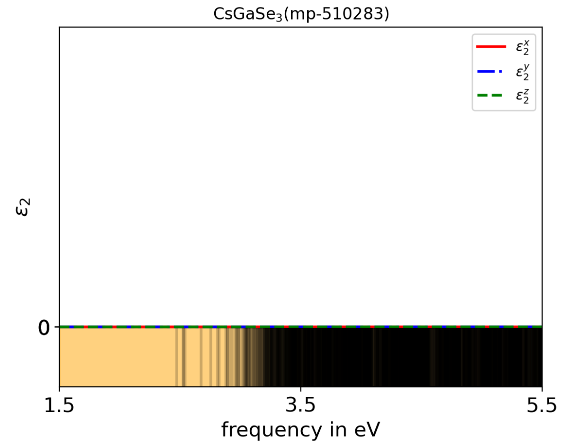
CsGaSe$_3$(mp-510283)
$\varepsilon_2^x$
$\varepsilon_2^y$
$\varepsilon_2^z$
$\varepsilon_2$
frequency in eV

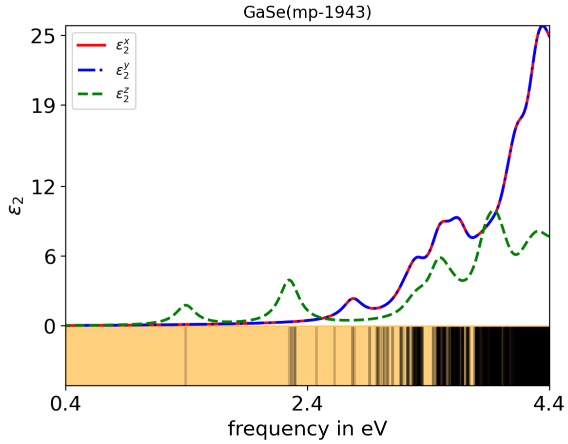
GaSe(mp-1943)
$\varepsilon_2^x$
$\varepsilon_2^y$
$\varepsilon_2^z$
$\varepsilon_2$
25
19
12
6
0
0.4
2.4
4.4
frequency in eV

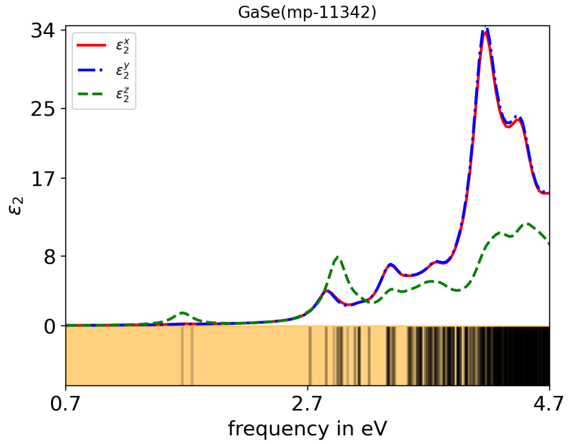
GaSe(mp-11342)
$\varepsilon_2^x$
$\varepsilon_2^y$
$\varepsilon_2^z$
$\varepsilon_2$
34
25
17
8
0
0.7
2.7
4.7
frequency in eV

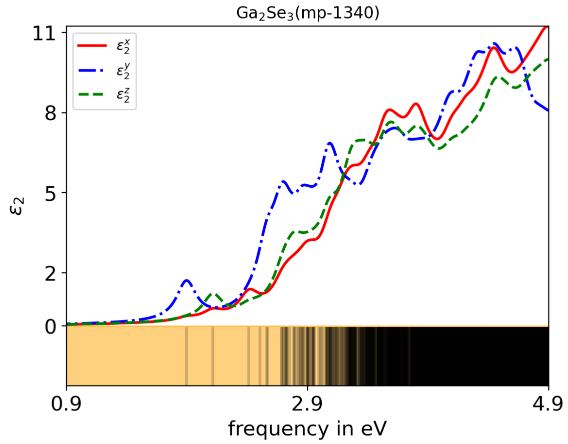
$Ga_2Se_3$(mp-1340)
$\varepsilon_2^x$
$\varepsilon_2^y$
$\varepsilon_2^z$
$\varepsilon_2$
11
8
5
2
0
0.9
2.9
4.9
frequency in eV

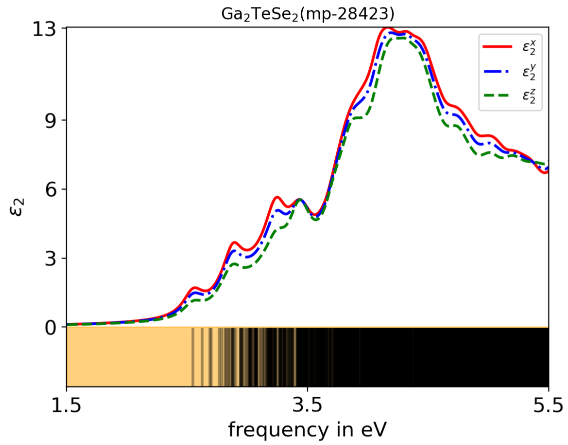
$Ga_2TeSe_2$(mp-28423)
$\varepsilon_2^x$
$\varepsilon_2^y$
$\varepsilon_2^z$
$\varepsilon_2$
13
9
6
3
0
1.5
3.5
5.5
frequency in eV

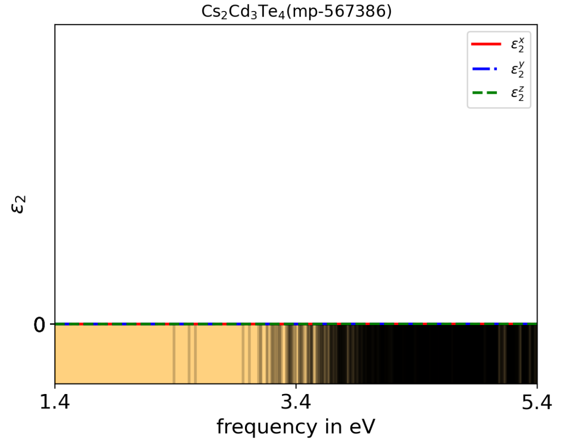
Cs$_2$Cd$_3$Te$_4$(mp-567386)
$\varepsilon_2^x$
$\varepsilon_2^y$
$\varepsilon_2^z$
$\varepsilon_2$
0
1.4
3.4
5.4
frequency in eV

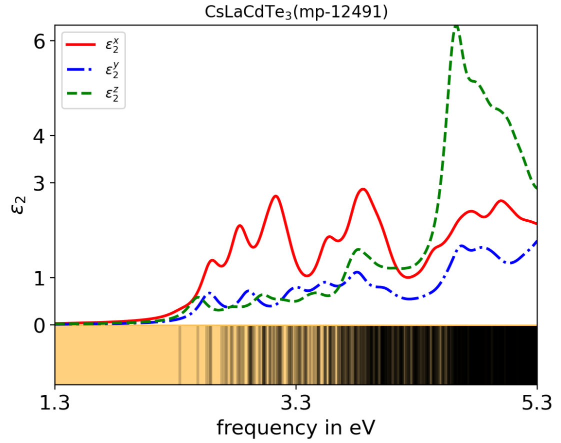
CsLaCdTe$_3$(mp-12491)
$\varepsilon_2^x$
$\varepsilon_2^y$
$\varepsilon_2^z$
$\varepsilon_2$
6
4
3
1
0
1.3
3.3
5.3
frequency in eV

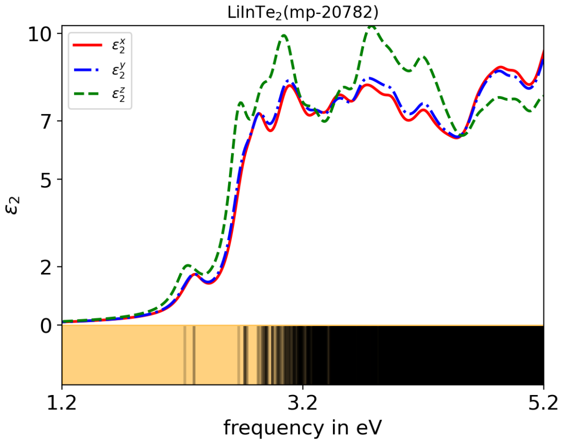
LiInTe$_2$(mp-20782)
$\varepsilon_2^x$
$\varepsilon_2^y$
$\varepsilon_2^z$
$\varepsilon_2$
10
7
5
2
0
1.2
3.2
5.2
frequency in eV

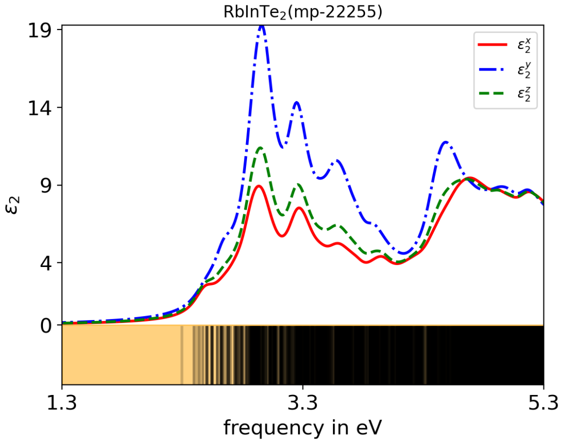
RbInTe$_2$(mp-22255)
$\varepsilon_2^x$
$\varepsilon_2^y$
$\varepsilon_2^z$
$\varepsilon_2$
19
14
9
4
0
1.3
3.3
5.3
frequency in eV

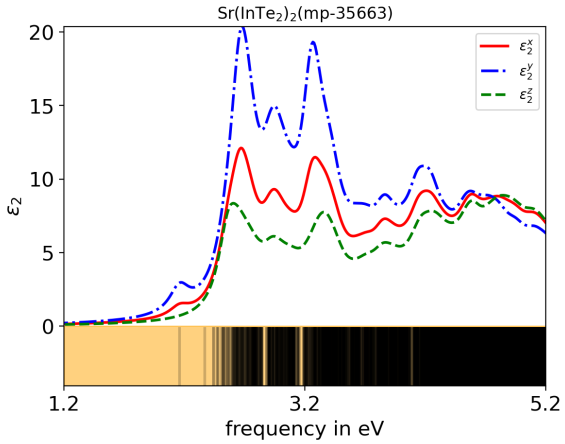
Sr(InTe$_2$)$_2$(mp-35663)
$\varepsilon_2^x$
$\varepsilon_2^y$
$\varepsilon_2^z$
$\varepsilon_2$
0
5
10
15
20
1.2
3.2
5.2
frequency in eV

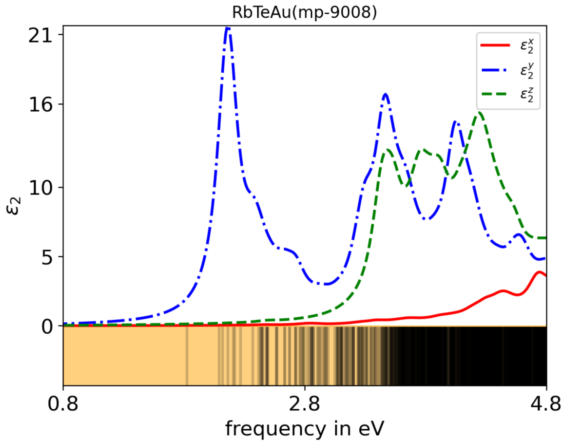
RbTeAu(mp-9008)
$\varepsilon_2^x$
$\varepsilon_2^y$
$\varepsilon_2^z$
$\varepsilon_2$
0
5
10
16
21
0.8
2.8
4.8
frequency in eV

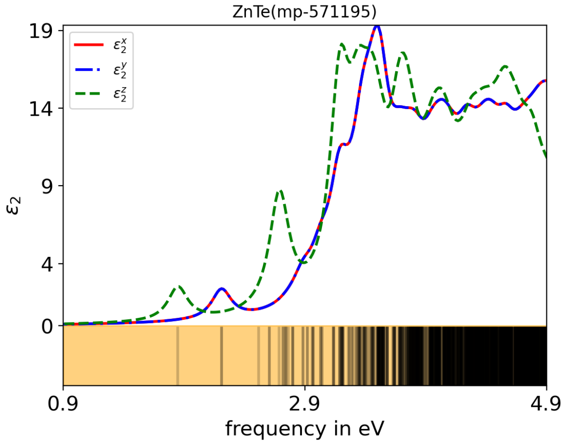
ZnTe(mp-571195)
$\varepsilon_2^x$
$\varepsilon_2^y$
$\varepsilon_2^z$
$\varepsilon_2$
0
4
9
14
19
0.9
2.9
4.9
frequency in eV

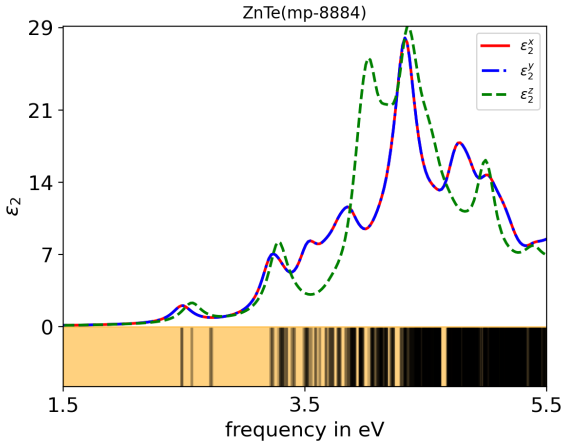
ZnTe(mp-8884)
$\varepsilon_2^x$
$\varepsilon_2^y$
$\varepsilon_2^z$
$\varepsilon_2$
0
7
14
21
29
1.5
3.5
5.5
frequency in eV

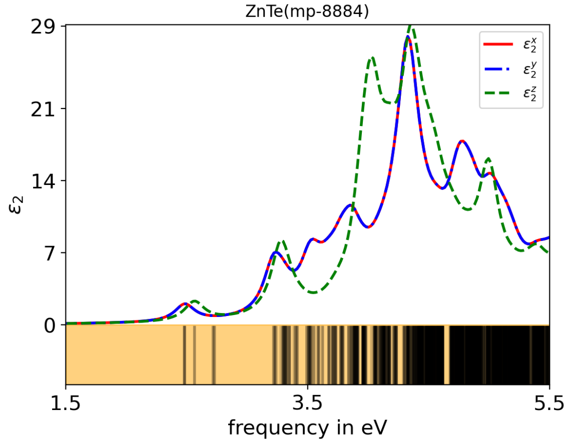
ZnTe(mp-8884)
$\varepsilon_2^x$
$\varepsilon_2^y$
$\varepsilon_2^z$
$\varepsilon_2$
29
21
14
7
0
1.5
3.5
5.5
frequency in eV

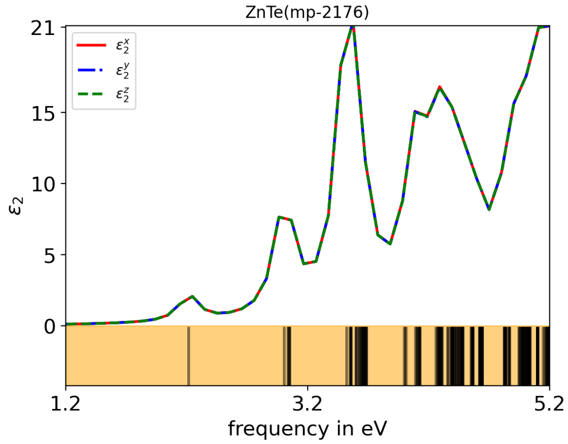
ZnTe(mp-2176)
$\varepsilon_2^x$
$\varepsilon_2^y$
$\varepsilon_2^z$
$\varepsilon_2$
21
15
10
5
0
1.2
3.2
5.2
frequency in eV

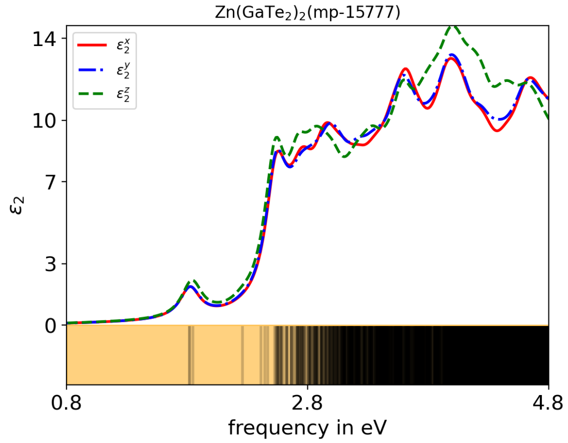
$Zn(GaTe_2)_2$(mp-15777)
$\varepsilon_2^x$
$\varepsilon_2^y$
$\varepsilon_2^z$
$\varepsilon_2$
14
10
7
3
0
0.8
2.8
4.8
frequency in eV

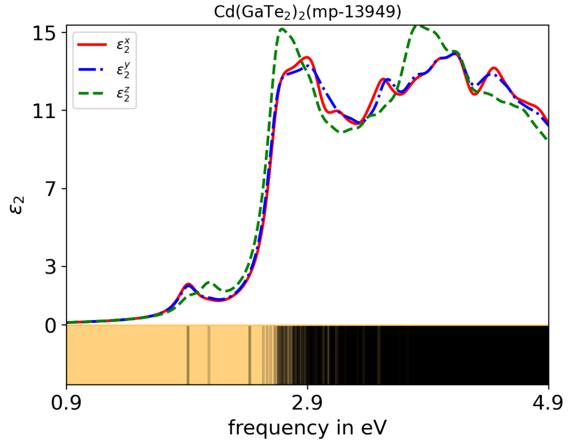
$Cd(GaTe_2)_2$(mp-13949)
$\varepsilon_2^x$
$\varepsilon_2^y$
$\varepsilon_2^z$
$\varepsilon_2$
15
11
7
3
0
0.9
2.9
4.9
frequency in eV

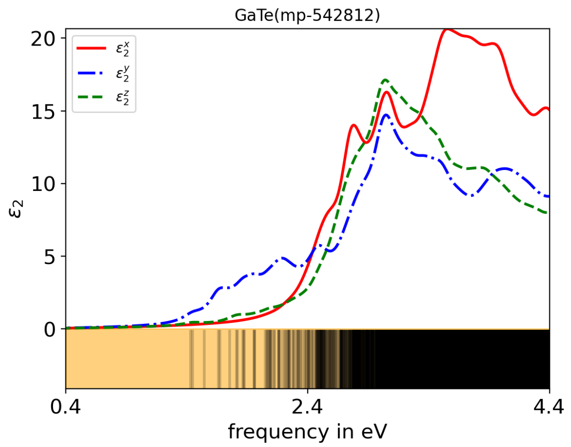
GaTe(mp-542812)
$\varepsilon_2$
frequency in eV
$\varepsilon_2^x$
$\varepsilon_2^y$
$\varepsilon_2^z$

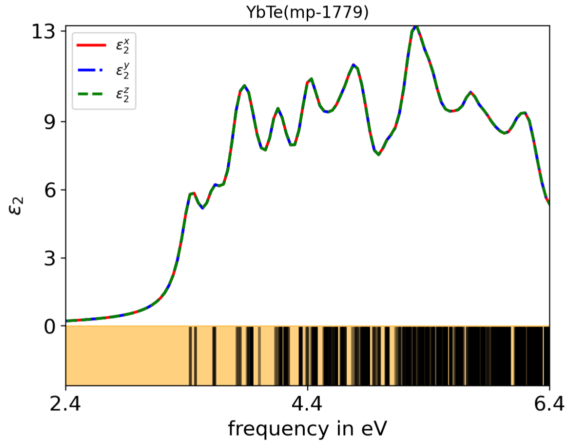
YbTe(mp-1779)
$\varepsilon_2$
frequency in eV
$\varepsilon_2^x$
$\varepsilon_2^y$
$\varepsilon_2^z$

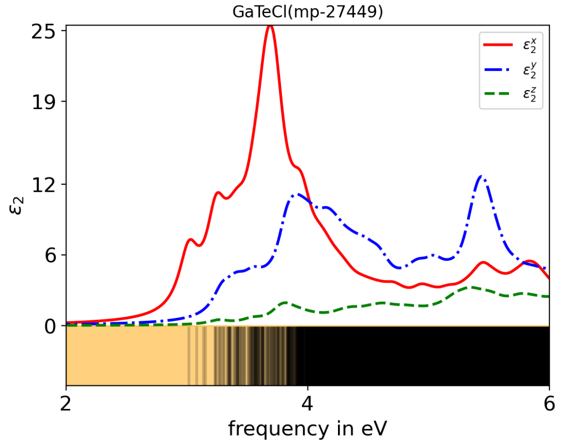
GaTeCl(mp-27449)
$\varepsilon_2$
frequency in eV
$\varepsilon_2^x$
$\varepsilon_2^y$
$\varepsilon_2^z$

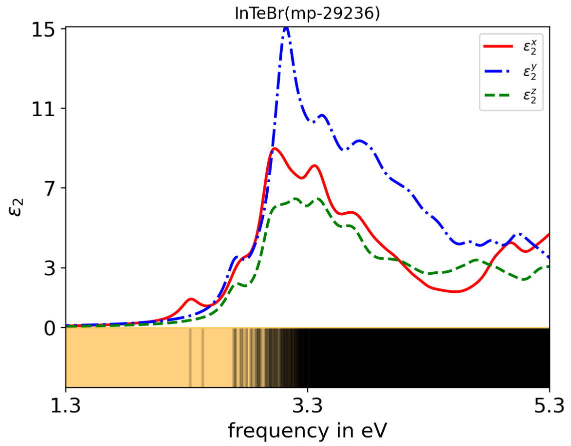
InTeBr(mp-29236)
$\varepsilon_2$
frequency in eV
$\varepsilon_2^x$
$\varepsilon_2^y$
$\varepsilon_2^z$

[1] Singh, A. K., Montoya, J. H., Gregoire, J. M. & Persson, K. A. Robust and synthesizable photocatalysts for $CO_2$ reduction: a data-driven materials discovery. *Nature communications* **10**, 1–9 (2019).
